# Supplementary material for: Optimisation of cyber insurance coverage with selection of cost effective security controls
Source: arXiv:2503.02706 source file (2025-03-04)
Supplement: Supplementary file 1 [file Additional.tex]

\begin{algorithm}[!th]
	\caption{Selecting the best set of countermeasures}\label{alg:main}
	\begin{algorithmic}[1]
		\Procedure{searchForOptimalInvesments}{$K$, $C$, $ \pi $, $\bar{R}$, $x_{limit}$}
		\Require $K$ \Comment{- a set of countermeasures}\\
		$c:K\mapsto \mathbb{N}$ \Comment{- cost function}\\
		$\pi:K\mapsto 2^{[0;1]}$ \Comment{- survival probability per threat function}\\
		$\bar{R}$ \Comment{- current Risk vector of $\mathbb{N}^{+}$ values}\\
		$x_{init}\in \mathbb{N}$ \Comment {- Investment Limit (optionally)}\\
		$C\in \mathbb{N}$ \Comment{the greatest common divisor for countermeasure cost}
		\Ensure \texttt{lowest $(\prod \pi(K_{i}|x))\times \bar{R} + x$ for optimal security investment $ x^* $ or within a given $ x $}
		\BState \emph{\textbf{Main Function}}:
		\Require ID of the countermeasure
		\State Call Initial Population Function
		\State Main Loop:
		\State: Crossover process:
		\State: Mutation process:
		\State: Run the loop for \textit{LIMIT}:
			\end{algorithmic}
		\begin{algorithmic}[1]
		\BState \emph{\textbf{Initial Population}}:
		\State Initialize the population of N number by removing ones that do not satisfy the following condition
		\State $ Perc = 100 $
		\For {i:=1 to N} \Comment N $ \rightarrow $ maximum number of chromosomes
		\State Generate Random Chromosome \Comment select only one countermeasure in the chromosome ensuring the best one if there are more than two countermeasures which have the same ID.
		\State Set all genes of chromosome as 0
		\State Replace the $ Perc $ percentage of them as 1
		\If {($x_{limit}$ $ > 0 $ \&\& $x_{limit}$ $ < U $)} 
		\State $ i:= i - 1 $ \Comment Remove the chromosome which does not satisfy/survive the condition
		\State $ Perc:= Perc - 1 $ \Comment Decrease the percentage of replacement
		\EndIf
		\EndFor \\
		\Return Generated Random Chromosomes
			\end{algorithmic}
		\begin{algorithmic}[1]
				\BState \emph{\textbf{Crossover:}}
		\State Make crossover between a randomly chosen chromosome and our selected chromosome by changing the half of them.
		
		\Require Current Chromosomes
		\For {i:=1 to N} \Comment N $ \rightarrow $ N: Number of current chromosomes
		\State j = rand(1, N) $ \rightarrow $ generate random number in range 1 to N
		\State nextGen = crossover i-th and j-th chromosome \Comment i-th chromosome's first half and j-th chromosome's second half genes
		\EndFor
		\State Call the Merge function (current and nextGen chromosomes)\\
		\Return Merged Chromosomes
		\BState \emph{\textbf{Mutation:}} \Comment Mutate the chromosomes for a given number of bits/genes
		\Require k
		\For {i:=1 to N} \Comment N $ \rightarrow $ N: Number of current chromosomes
		\State Replace the k number of random bits in the chromosome
		\State nextGen = mutated i-th chromosome	
		\EndFor
		\State Call the Merge function (current and nextGen chromosomes)\\
		\Return Merged Chromosomes
		\BState \emph{\textbf{Merge Function}}:
		\Require Current chromosomes, nextGen chromosomes
		\State \textbf{Append} Current chromosomes \textbf{to} nextGen chromosomes \Comment merge the two lists of chromosomes
		\State \textit{weight} = $(p(K_{i}|x))\times \bar{R} + x$
		\State \textbf{Sort} Current chromosomes by their \textit{weight} \Comment z to a way is used to sort the chromosomes 
		\State Select 60\% of chromosomes as good and rest as a random
		\EndProcedure
	\end{algorithmic}
\end{algorithm}

\begin{algorithm}[!th]
	\caption{Main Function of the GA algorithm}\label{alg:MainFuncs}
	\begin{algorithmic}[1]
		\Procedure{MainFunction}{$K$, $c$, $ \pi $, $\bar{R}$, $x_{limit}$, $ b $, $ LIMIT $, $ {Perc} $}
		\Require 
		$K$ \Comment{- a set of countermeasures}\\
		$c:K\mapsto \mathbb{N}$ \Comment{- cost function}\\
		$\pi:K\mapsto 2^{[0;1]}$ \Comment{- survival probability per threat function}\\
		$\bar{R}$ \Comment{- current risk vector of $\mathbb{N}^{+}$ values}\\
		$x_{limit}\in \mathbb{N}$ \Comment {- investment limit}\\
		$b \in \mathbb{N}$ \Comment {- a unique number assigned to each countermeasures}\\
		$LIMIT \in \mathbb{N}$ \Comment {- a constant value to run the GA}\\
		$Perc \in \mathbb{N}$ \Comment {- Percentage}
		\Ensure \texttt{lowest $(\prod \pi(K_{i}|x))\times \bar{R} + x|x_{limit}$ } \Comment for optimal security investment $ x $ or within a given $ x_{limit} $
		\BState \emph{\textbf{Check the inputs}}:
		\State Return acknowledgement message
		\BState \emph{\textbf{Call Initial Population Function}}:
		\BState \emph{\textbf{New Population}}: $ \rightarrow $ Loop for \textit{LIMIT}:
		\State Crossover process:
		\State Mutation process:
		\State Merge process:
		\EndProcedure
	\end{algorithmic}
\end{algorithm}

\\
\begin{algorithm}[!th]
	\caption{Initial Population and Fitness Assignment of the GA algorithm}\label{alg:Init1}
	\begin{algorithmic}[1]
		\Procedure{InitialPopulation}{$K$, $c$, $ \pi $, $\bar{R}$, $x_{limit}$, $ b $, $ LIMIT $, $ {Perc} $}
		\State $ Perc = 100 $
		\For {i:=1 to N} \Comment N $ \rightarrow $ maximum number of chromosomes
		\State Generate Random Chromosome
		\If {$ b > 0 $}
		\State Select a better chromosome among the same ID countermeasures
		\EndIf
		\State Set all genes of chromosome as 0
		\State Replace the $ Perc $ percentage of them as 1
		\If {($x_{limit}$ $ > 0 $ \&\& $x_{limit}$ $ < U $)} 
		\State $ i:= i - 1 $ \Comment Remove the chromosome which does not satisfy/survive the condition
		\State $ Perc:= Perc - 1 $ \Comment Decrease the percentage of replacement
		\EndIf
		\EndFor \\
		\Return Generated Random Chromosomes
		\EndProcedure
	\end{algorithmic}
\end{algorithm}

\begin{algorithm}[!th]
	\caption{Creation of New Population}\label{alg:NewPop}
	\begin{algorithmic}[1]
		\Procedure{NewPopulation}{$K$, $c$, $ \pi $, $\bar{R}$, $x_{limit}$, $ b $, $ LIMIT $, $ {Perc} $, $N$, $e$}
		\BState \emph{\textbf{Crossover:}}
		\State Make crossover between a randomly chosen chromosome and our selected chromosome by changing the half of them.
		
		\Require Current Chromosomes
		\For {i:=1 to N} \Comment N $ \rightarrow $ N: Number of current chromosomes
		\State j = rand(1, N) $ \rightarrow $ generate random number in range 1 to N
		\State nextGen = crossover i-th and j-th chromosome \Comment i-th chromosome's first half and j-th chromosome's second half genes
		\EndFor
		\State Call the Merge function (current and nextGen chromosomes)\\
		\Return Merged Chromosomes
		\BState \emph{\textbf{Mutation:}} \Comment Mutate the chromosomes for a given number of bits/genes
		\Require e
		\For {i:=1 to N} \Comment N $ \rightarrow $ N: Number of current chromosomes
		\State Replace the k number of random bits in the chromosome
		\State nextGen = mutated i-th chromosome	
		\EndFor
		\State Call the Merge function (current and nextGen chromosomes)\\
		\Return Merged Chromosomes
		\BState \emph{\textbf{Merge Function}}:
		\Require Current chromosomes, nextGen chromosomes
		\State \textbf{Append} Current chromosomes \textbf{to} nextGen chromosomes \Comment merge the two lists of chromosomes
		\State \textit{weight} = $(p(K_{i}|x))\times \bar{R} + x$
		\State \textbf{Sort} Current chromosomes by their \textit{weight} \Comment z to a way is used to sort the chromosomes 
		\State Select 60\% of chromosomes as good and rest as a random
		\EndProcedure
	\end{algorithmic}
\end{algorithm}

\begin{algorithm}[!th]
	\caption{Selecting the best set of countermeasures}\label{alg:main1}
	\begin{algorithmic}[1]
		\Procedure{searchForOptimalInvesments}{$K$, $c$, $\pi$, $\bar{F}$, $\bar{L}$, $x_{init}$, $pr_{init}$, C}
		\Require $K$ \Comment{- a set of countermeasures}\\
		$c:K\mapsto \mathbb{N}$ \Comment{- cost function}\\
		$\pi:K\mapsto 2^{[0;1]}$ \Comment{- survival probability per threat function}\\
		$\bar{F}
		$ \Comment{- frequency vector of $\mathbb{R}^{+}$ values}\\
		$\bar{L}$ \Comment{- single loss expectency vector of $\mathbb{N}^{+}$ values}\\
		$x_{init}\in \mathbb{N}$ \Comment {- initial investments}\\
		$\bar{pr}_{init}$ \Comment{- initial overall probability of survival vector of values from $[0;1]$} \label{line:LastDefinition}\\
		$C\in \mathbb{N}$ \Comment{the greatest common divisor for countermeasure cost}
		\Ensure \texttt{lowest $(\bar{F}\cdot \bar{pr}(K_{i}|x))\times \bar{L} + x$ for optimal security investment $ x^* $}
		\State $ exp \Leftarrow (\bar{F}\cdot\bar{pr}_{init})\times\bar{L} + x_{init}$  \Comment{Remember the initial expenditure as optimal} \label{line:firstA}
		\State $P^{*}_{min}=\bar{F}\cdot \left[ \prod_{\forall k\in K} \bar{\pi}(k)\right])\times \bar{L}$
		\State $ x^* \Leftarrow 0 $ \Comment{Optimal Investment starts with $x_{init}$} 
		\State $\forall j~T[j][0] \Leftarrow~\{\bar{pr}_{init}\}$ \Comment{a dynamic matrix of optimal probabilities. Add new (and the first) column $x=x_{init}$, with just one vector $\bar{pr}_{init}$} \label{line:Tinit}
		\State $ x \Leftarrow C $ \label{line:xinit} \Comment{the size of set $K$}
		\State $ n_{k} \Leftarrow |K| $ \label{line:finInit}
		\While{$x+x_{init}  \le exp-P^{*}_{min} $} \Comment{Do while $x$ is below the optimal expenditure} \label{line:While}
		\State $\forall j~T[j][x] \Leftarrow~\{\bar{pr}_{init}\}$ \Comment{Add new column x, initialised with vector $\bar{pr}_{init}$}
		\For{$j \Leftarrow 1, n_{k}$} \Comment{for all countermeasures} \label{line:For}
		\If{($c(k_j)$ $\leq$ $x$ )} \label{line:CompareCost} \Comment{check the cost limit}
		\State $ T[j][x] \Leftarrow non-dominant 
		\left\{ 
		\begin{array}{l}
		\bigcup\limits_{\forall l} \bar{\pi}(k_j) \cdot T[j-1][x-c(k_j)][l]\\
		T[j-1][x] 
		\end{array}
		\right.$ \Comment{store all non-dominant vectors comparing two sets: with new control and without.} \label{line:Selection}
		\Else
		\State $T[j][x] \Leftarrow T[j-1][x]$ \Comment{continue without adding new control $j$ } \label{line:HighCost}
		\EndIf    
		\EndFor
		\For{$l\Leftarrow 0,|T[n_{k}][x]|$} \Comment{for all vectors stored in $T[n_{k}][x]$}
		\If{$ (\bar{F}\cdot T[n_{k}][x][l])\times \bar{L} + x + x_{init}  < exp $} \Comment{reduced the expenditure?} \label{line:CheckCondition}
		\State $ exp \Leftarrow \bar{F}\cdot T[n_{k}][x][l])\times \bar{L} + x + x_{init} $ \Comment{Store this expenditure as optimal} \label{line:reSetCondition}
		\State $x^* \Leftarrow x$ \Comment{Remember these investments as optimal} \label{line:reSetOptimal}
		\EndIf
		\EndFor
		\State $ x \Leftarrow x + C $
		\EndWhile\\
		\Return [$ exp, x^*$]
		\EndProcedure
	\end{algorithmic}
\end{algorithm}
